# Supplementary material for: Linear-quadratic stochastic delayed control and deep learning resolution
Source: arXiv:2102.09851 source file (2021-02-24)
Supplement: Supplementary file 1 [file appendice.tex]

%%%%%%%%%%%%%%%%%%%%%%%%%%%%%%%%%%%%%%%%

\section{Generic verification result pour le gros modèle}

Given the linear-quadratic structure of the problem, it is natural to consider a  candidate optimal value process 
$(V^\c_t)_{t \leq T}$ of linear-quadratic form in the state variables $(X^\c_t, X^\c(t), \c(t))$ {\green corriger/definir notation} that is 
\bes{
    %\label{eq:value_fun}
    V^\c_t =& E_1^t X_t^2 + \intd X_s^2 E_2^t(t-s-\delta) ds  + \intdd X_sX_u E_3^t(t-s-\delta, t-u-\delta)  ds du \\
    & + X_t \intd X_s E_4^t(t-s-\delta) ds \\
    &  +  2\bigg\{ \intdd X_s \c_u E_5^t(t-s-\delta, t-u-\delta)dsdu \\
    &+  X_t \intd \c_s E_6^t(t-s-\delta) ds +  \intd \c_s X_s E_7^t(t-s-\delta) ds \bigg\} \\
    &  + \intd \c^2_s E_8^t(t-s-\delta) ds+\intdd \c_s\c_u E_9^t(t-s-\delta, t-u-\delta)  ds du\\,
}
where the functions $t \mapsto E^t_i$ satisfy $E^T_1=P, E^T_i=0$ for $2\leq i\leq 9$ and are solutions, in a suitable sense defined in \ref{def:sol_E_i}, of the following system of equations for almost any $(t,s,u) \in [0,T] \times [-\delta, 0]^2$

\bes{
    %\label{eq:E_i}
	     \dot{E}_1^t  + Q +E_1^t(2B + D^2) + E_2^t(-\delta) + E^t_4(-\delta)=&\frac{\left(E_1(C+FD) + E^t_7(-\delta)+E^t_6(-\delta)\right)^2}{\hat{N}_t}, \\
	     (\partial_t + \partial_s) E_2^t(s) =& 0 \\
	     (\partial_t +\partial_s + \partial_u) E_3^t(s, u) =& \frac{E_5^t(s,-\delta)E_5^t(-\delta,u)}{\hat{N}_t} \\
	      (\partial_t + \partial_s + B)E_4^t(s) + E_3^t(-\delta) =&\frac{ (E_1^t(C+FD)+ E_6^t(-\delta)+ E_7^t(-\delta))E_5^t(s-\delta)}{\hat{N}_t} \\
	     (\partial_t + \partial_s + \partial_u)E_5^t(s, u) =& \frac{E_5^t(s,-\delta)(E_9^t( -\delta,u)+CE_6^t(u))}{\hat{N}_t} \\
	     \left( (\partial_t + \partial_s + B)E_6^t(\cdot) +E_5(-\delta, \cdot)\right)(s) =& \frac{\left(E_1^t(C+FD)+E_6^t(-\delta)+E_7^t(-\delta)\right)(E_9(-\delta, u) + CE_6^t(u))}{\hat{N}_t} \\
	     (\partial_t + \partial_s)E_7^t(s) =&0 \\
	     (\partial_t + \partial_s) E_8^t(s)=&0\\
	     (\partial_t + \partial_s + \partial_u) E_9^t(s,u) =& \frac{(E_9^t(-\delta,s)+CE_6^t(s))(E_9^t(u,-\delta)+CE_6^t(u))}{\hat{N}_t}. \\
	}   
With the following boundary conditions for almost any $t, s\in [0,T) \times [-\delta, 0]$
\bes{
    %\label{eq:E_i_boudary_cond}
     E_1^t \tilde{D}^2 - E_2^t(0)=& \frac{\left(\tilde{D}F E_1^t\right)^2}{\hat{N}_t}  \\
	      \left(\tilde{B}E_4^t(\cdot) - E_3^t(0, \cdot)-E_3^t(\cdot, 0) \right) (s) =& \frac{(D\tilde{F}E^t_1)E^t_5(s,-\delta)}{\hat{N}_t}\\
	      2( \tilde{B} +  D\tilde{D})  E_1^t - E_4^t(0) =& \frac{\tilde{D}F E_1^t(E_1^t(C+FD)+ E_6^t(-\delta)+ E_7^t(-\delta))}{\hat{N}_s} \\
	      2(\tilde{C}+ D \tilde{F})E_1^t - E_6^t(0) =& \frac{F\tilde{F}E_1^t (E_1^t(C+FD)+ E^t_7(-\delta)+ E^t_6(-\delta))}{\hat{N}_s} \\
	      \tilde{D} \tilde{F} E_1^t - E_7^t(0) =& \frac{F^2 \tilde{D}\tilde{F} (E_1^t)^2}{\hat{N}_s} \\
	      \left( \tilde{C} E_4^t(\cdot) - E_5^t(\cdot, 0)\right)(s) =& \frac{ F\tilde{F}E_1^t E_5^t(s,-\delta) }{\hat{N}_t} \\
	      \left(\tilde{B}E_6^t(\cdot)- E_5^t(0, \cdot) \right)(s ) =& \frac{F\tilde{D}E_1^t(E_9^t(-\delta, s)+ CE_6^t(s)))}{\hat{N}_t}\\
	      \tilde{F}^2 E_1^t - E_8^t(0) =& \frac{(F \tilde{F} E_1^t)^2}{\hat{N}_t}\\
	       \left( \tilde{C} E_6^t(\cdot) - E_9^t(\cdot, 0) - E_9^t(0, \cdot) \right) (s)=& \frac{F\tilde{F} E^1_t(E_3^t(-\delta, s)+CE_6^t(s))}{\hat{N}_t}, \\
}
where $\hat{N}_t  = N + F^2 E_1^t + E_8^t(-\delta)$ for $t\in [0,T]$. The following definition specify the concept of solution to the system \eqref{eq:E_i}.
\begin{definition}
%\label{def:sol_E_i}
By solution to the system \eqref{eq:E_i}-\eqref{eq:E_i_boudary_cond} we mean a 9-uplets $(E_i)_{1 \leq i \leq  9}$ {\green of functions of bounded variations} satisfing almost everywhere the set of equation \eqref{eq:E_i} and such that $\hat{N}_t > 0$ for any $t\in [0,T]$.
\end{definition}

\begin{proposition}
%\label{prop:properties_value}
The set  of equations $\eqref{eq:E_i}$ has a unique solution. This solution is uniformly bounded and uniformly lipshitzian in each of its variables. Furthermore 
\begin{enumerate}
    \item $ V_t \to_{t \to \c} PX_T^2$ \label{item:limit_V_T}
    \item $\hat{N} >0$ \label{item:N_positive}
\end{enumerate}
\end{proposition}
\begin{proof}
   {\green  etendre Alekal 1978}
\end{proof}

\bes{
    %\label{eq:optimal_control_final}
    \c^*_t =&-(N + E_1^t F^2 + E_8^t(-\delta) )^{-1} \bigg\{ X_t\left(E_1^t(C+FD) + E^t_6(-\delta) + E^t_7(-\delta) \right) \\
    &+ X_{t-\delta} (\tilde{D}F E_1^t) + \int_{t-\delta}^t X_s E^t_5(t-s-\delta)  ds \\
    &+ \int_{t-\delta}^t \c_s (E^t_9(-\delta, t-s-\delta) + C E^t_6(t-s-\delta)) ds+\c_{t-\delta} (F\tilde{F}E^t_1) \bigg\}.
}

\begin{theorem}[Verification Theorem]
%\label{T:verif}
Assume that 
\begin{enumerate}
    \item The set of equations \eqref{eq:E_i} admits solution in the sense of \ref{def:sol_E_i}; \label{T:verif:i}
    \item There exists an admissible control satisfying \eqref{eq:optimal_control_final}. \label{T:verif:ii}
\end{enumerate}
Then the optimization problem admits \eqref{eq:optimal_control_final} as an optimal feedback  control and the value function is given by \eqref{eq:value_fun}.
\end{theorem}
\begin{proof}
    \fbox{draft}
   For any $\c \in \mathcal{A}$, let us  define the  continuous process
   \bes{
    M_t^\c &= \int_0^t f(X_s^\c, \c_s) ds + V_t - \int_0^t \hat{N}_s (\c_s - \c_s^*)^2 ds.
   }
   We prove that $M^{\alpha}$ is a local martingale by means of It\^o's formula and a completion of squares in $\c$.
	\bes{
	d V_t =& \Bigg\{\textbf{1}_t X^2_t  + \textbf{2}_t X_\td^2 +  \intdd \textbf{3}_t(s,u) X_s X_u ds du + \intd \textbf{4}_t(s) X_s^2 ds  \\
	&+ X_\td \intd \textbf{5}_t(s) X_s ds +  X_t \intd \textbf{6}_t(s) X_s ds + \textbf{7}_t X_t X_\td \\
	&+2 \bigg( \textbf{8}_t X_t\c_t+ \textbf{9}_t X_t\c_\td+ \textbf{10}_t X_\td \c_{t} + \textbf{11}_t X_\td\c_\td \\
	&+ \c_t \textbf{12}_t(s) \intd X_s ds + \intd\textbf{13}_t(s) X_s \c_s ds +  \intdd \textbf{14}_t(s,u) X_s \c_u ds du\\
	&   +  X_t \intd \textbf{15}_t(s) \c_s ds +  \c_\td \intd \textbf{16}_t(s) X_s ds +  X_\td \intd \textbf{17}_t(s) \c_s ds \bigg) \\
	&+  \textbf{18}_t  \c_t^2 + \textbf{19}_t \c_t \c_\td + \textbf{20}_t \c_\td^2  +  \c_\td \textbf{21}_t(s) \intd \c_s ds + \c_t \intd \textbf{22}_t(s) \c_s ds \\
	&+   \intd \textbf{23}_t(s) \c^2_s ds + \intdd \textbf{24}_t(s,u) \c_s \c_u dsdu\Bigg\}dt + Z^\c_t dW_t,
	}
	where 
	\begin{align}
	    &\textbf{1}_t = \dot{E}_1^t  + E_1^t(2B + D^2) + E_2^t(-\delta) + E^t_4(-\delta), && \textbf{2}_t = E_1^t \tilde{D} - E_2^t(0) \\
	    &\textbf{3}_t(s,u) = (\partial_t +\partial_s + \partial_u) E_3^t(t-s-\delta, t-u-\delta), &&  \textbf{5}_t(s) = \left(\tilde{B}E_4^t(\cdot) - E_3^t(0, \cdot)-E_3^t(\cdot, 0) \right) (t-s-\delta) \\
	     &\textbf{4}_t(s) = (\partial_t + \partial_s) E_2^t(t-s-\delta) && \textbf{7}_t = 2( \tilde{B} +  D\tilde{D})  E_1^t - E_4^t(0)\\
	     &\textbf{6}_t(s) = (\partial_t + \partial_s + B)E_8^t(t-s-\delta) E_4^t + E_3^t(-\delta)  &&\textbf{8}_t =  (C + FD)E_t^1 + E_7^t(-\delta) + E_6^t(-\delta) \\
	     &\textbf{13}_t(s) = (\partial_t + \partial_s)E_7^t(t-s-\delta) && \textbf{9}_t = 2(\tilde{C}+ D \tilde{F})E_1^t - E_6^t(0) \\
	     &\textbf{14}_t(s,u) =  (\partial_t + \partial_s + \partial_u)E_5^t(t-s-\delta, t-u-\delta) && \textbf{10}_t = F \tilde{D} E_1^t  \\
	      &\textbf{15}_t(s) =\left( (\partial_t + \partial_s + B)E_6^t(\cdot) +E_5(-\delta, \cdot)\right)(t-s-\delta)   && \textbf{11}_t = \tilde{D} \tilde{F} E_1^t - E_7^t(0) \\
	         &\textbf{23}_t(s) = (\partial_t + \partial_s) E_8^t(t-s-\delta) &&  \textbf{12}_t(s) = \left(E_5^t(\cdot, -\delta) + CE_4^t(\cdot) \right)(t-s-\delta)\\
	     &\textbf{24}_t(s,u) = (\partial_t + \partial_s + \partial_u) E_9^t(t-s-\delta, t-u-\delta) &&  \textbf{16}_t(s) = \left( C E_4^t(\cdot) - E_5^t(\cdot, 0)\right)(t-s-\delta ) \\
	    &\textbf{18}_t =  F^2 E_1^t(-\delta) + E_7^t(-\delta) && \textbf{17}_t(s) = \left(\tilde{B}E_6^t(\cdot)- E_5^t(0, \cdot) \right)(t-s-\delta )\\
	    & \textbf{20}_t = \tilde{F}^2 E_1^t - E_8^t(0) && \textbf{19}_t = 2 F \tilde{F} E_1^t\\
	     &\textbf{22}_t(s) = \left( E_9^t(-\delta, \cdot) + C E_6^t(\cdot) \right) (t-s-\delta)  && \textbf{21}_t(s) =\left( C E_6^t(\cdot) - E_9^t(\cdot, 0) - E_9^t(0, \cdot) \right) (t-s-\delta) \\
	\end{align}
	and 
	\bes{
	    Z^\c_t = \sigma(X_t^{\c}, X_\td^{\c},\c_{t},\c_{\td}) \left( 2X_t^{\c} E_1^t +\intd X^\c_s E_4^t(t-s-\delta) ds  +\intd \c_s E_6^t(t-s-\delta) ds  \right).
	}
	Using the set of constraints $\eqref{eq:E_i}$ together with \eqref{eq:optimal_control} and a completion of squares in $\c$ yield
	\bes{
	    dM^\c_t = Z^\c_t dW_t.
	}
	Note that the stochastic integral $\int_0^. Z_s^\c dW_s$ is well defined since $X^\c$ is continuous, $\c \in L_{\F}^{2,loc}([0,T], L^2(\Omega, \R^N))$ and $E_1, E_4, E_6$ are bounded. Furthermore it is a local martingale. Let $\{\tau_k\}_{k\geq 1}$ be a localizing increasing sequence of stopping times  converging to $T$. Then, for any $k\geq 1$
	\bes{
	    \E\left[M_{T \wedge \tau_k}^\c\right] = M_0^\c,
	}
	which is equivalent to
	\bes{
	   \E \left[ \int_0^{T \wedge \tau_k} f(X_s^\c, \c_s)ds + V_{T \wedge \tau_k}) \right] =& V_0 + \E \left[ \int_0^{T\wedge \tau_k} \hat{N}_s(\c_s - \c_s^*)^2ds\right]
	}
	Since $\alpha \in \mathcal A$, $X^{\c}$ satisfies so that $\E\left[\sup_{t\leq T}  | X^{\c}_t|^2\right]<\infty$. An application of the dominated convergence theorem {\green attention cela ne semble pas évident puisque les $E_i$ semblent converger vers $0$ dans $L^1$. } on the left term combined with the monotone convergence theorem on the right term yields, as $k \to \infty$

	\bes{
	   \E \left[ \int_0^{T} f(X_s^\c, \c_s)ds + g(X_{T}) \right] =& V_0 + \E \left[ \int_0^{T} \hat{N}_s(\c_s - \c_s^*)^2ds\right],
	}
	where we used proposition \ref{prop:properties_value}-\ref{item:limit_V_T}.	Since $\hat{N}_s$ is positive {\green to justify}, we obtain that the optimal strategy is given by $\c^*$ and that the optimal value is equal to $V_0$.
\end{proof}

\begin{lemma}
    Assume that there exists a bounded solution to \eqref{}. Then \eqref{eq:optimal_control_final} is an admissible control.
\end{lemma}

%%%%%%%%%%%%%%%%%%%%%%%%%%%%%%%%%%%%%%%%

\subsection{Portfolio liquidation with temporary and permanent market impact}
{\green je ne sais plus ou trouver le modele qui pourrait nous interesser}\\
{\red Article d'Huyên et Matteo, \cite{basei2017linear}, à priori. Quid du "linear permanent impact due to the average trading of all market participants", on considère que tous les traders ont le même retard?} {\green Perso je propose de reprendre le modele sans mean-field, sinon cela donne du mean-field avec delay ce qui va alourdir pas mal le truc}

We now focus on the problem of portfolio liquidation with permanent price impact due to similar participants, treated in \cite{basei2017linear} in the case with no delay. This problem derives from the classical problem of portfolio liquidation initiated in \cite{almgren2001optimal}. We consider a finite-horizon model and compute the optimal control by Theorem \ref{T:verif}.\\
A trader has to liquidate a certain number of shares $x_0 \geq 0$ before a terminal time $T > 0$. She controls the trading speed $\alpha_t$ through time and her inventory $X_t^\alpha$ evolves according to this trading speed with a delay $\delta$, due to the latency of her communication with the stock exchange platform. Her inventory thus evolves according to
\begin{equation}
    \label{eq:inventory}
    X_t^\alpha = x_0 + \int_0^{t-\delta} \alpha_s ds,
\end{equation}
for $0 \leq t \leq T$. The price $S = S^\alpha$ of the asset is subject to a permanent market impact generated by the trading of the investor. The stock price is given by
\begin{equation}
    \label{eq:stock_price}
    S_t^\alpha = S_t^0 + \nu \int_0^{t-\delta} \alpha_s ds,
\end{equation}
where $S_0$ is an exogenous $\F$-adapted process representing the asset price in absence of trading, and $\nu \geq 0$ is a positive parameter modeling the linear permanent impact due to the average trading of all market participants. The objective of the investor is then to minimize, over her trading speed $\alpha$, the expected total liquidation cost
\begin{equation}
    \label{eq:liquid_cost1}
    J(\alpha)=\E \left[ \int_0^T \left( q\left(X_t^\alpha \right)^2 +\alpha_{t-\delta} \left( S_t^\alpha + \eta \alpha_{t-\delta} \right) \right)dt + p\left(X_T^\alpha \right)^2  \right],
\end{equation}

where $q \geq 0$ is a penalty parameter on the current inventory, $p \geq 0$ is a parameter penalizing the remaining inventory at maturity $T$ and $\eta > 0$ is a constant parameter modelling the linear temporary market impact. Due to the delay between the traders decision and its effect on the market, the linear temporary market impact at time $t$ is created by the trading speed chosen at time $t-\delta$ and is thus equal to $S_t^\alpha + \eta \alpha_{t-\delta}$. At time $t$, the execution price of a market order corresponding to the trading speed $\alpha$ is then equal to $\alpha_{t-\delta} \left( S_t^\alpha + \eta \alpha_{t-\delta} \right) dt$. Since $S_t^\alpha = S_t^0 + \nu\left(X_{t-\delta} -x_0  \right)$, the cost functional can be rewritten as 

\begin{equation}
    \label{eq:liquid_cost2}
    J(\alpha)=\E \left[ \int_0^T \left( q\left(X_t^\alpha \right)^2 + \eta \alpha_{t-\delta}^2 + \left( S_t^0 -\nu x_0 \right)\alpha_{t-\delta} + \nu \alpha_{t-\delta} X_{t-\delta}^\alpha \right)dt + p\left(X_T^\alpha \right)^2  \right].
\end{equation}
{\green là on a un problème mean-field avec delay, ca se resout aussi mais je sais pas si on a envie de rentrer la dedans. Dans $S_t^\c$ je pense que l'on pourrait retirer l'esperance sur le $\c$}

%%%%%%%%%%%%%%%%%%%%%%%%%%%%%%%%%%%%%%%%
